# Supplementary material for: Enhancing Review Comprehension with Domain-Specific Commonsense
Source: arXiv:2004.03020 source file (2020-04-06)
Supplement: Supplementary file 1 [file appendix.tex]

Specifically, we first collected 7592 real customer questions from TripAdvisor, and used reviews from the OpinRank dataset~\cite{ganesan2012opinion}, which contains around 259,000 reviews from TripAdvisor too. To increase the chances of finding non-trivial QA pairs, we focused on questions on three common hotel aspects: parking, breakfast and pool. Take the parking aspect as an example. We search for parking questions and group them based on the sub-topics, such as parking fee or parking safety, so that we will not provide redundant questions for human annotation. We also selected candidate reviews that mention parking at least three times, to make it more adversarial for machine learning models. Then we launch our first crowd-sourcing task for detecting relevant reviews for each sub-topic. In this task, we presented a review to a human annotator, along with all the possible sub-topics, and asked the human annotator to select sub-topics mentioned in the review. The result of this task is a set of ({\it review} {\it relevant sub-topic}) pairs. After this, we launched a second crowd-sourcing task. In this task, for each ({\it review} {\it relevant sub-topic}) pair, we found concrete questions under the sub-topic. If the {\it review} does not share the noun phrases in the question -- such as ``free parking'' here -- we presented the ({\it review} {\it concrete question}) to the crowd-sourcing annotators for answer annotation. For instance, given {``The location is good. Parking takes 3 dollars'', ``parking fee''}, and a concrete question ``Do you have free parking?'', we give the crowd-sourcing annotators (``The location is good. Parking takes 3 dollars'', ``Do you have free parking?''), and asked them a sentence span in {\it review} that answers the question, if there is any. In this task, the annotators need to rely on their commonsense to select the answer, because the words in the question do not appear in the review. The result of the second crowd-sourcing task is our QA dataset.  In our example, the answer span is ``Parking takes 3 dollars''. 
In both crowd-sourcing tasks, three crowds-sourcing annotators made judgements on each data entry for quality control. If at least two annotators have the same annotation, that annotation is taken as the golden one.
